# Supplementary material for: Including Everyone, Everywhere: Understanding Opportunities and Challenges of Geographic Gender-Inclusion in OSS
Source: arXiv:2010.00822 source file (2021-09-16)
Supplement: Supplementary file 1 [file appendix-only.tex]

\documentclass[10pt,journal,compsoc]{IEEEtran}

\input{utils.tex}
\input{aliases.tex}

\begin{document}
\appendices
\subfile{appendix}

\bibliographystyle{IEEEtran}
\bibliography{global_dev_study}
\end{document}
